# Supplementary material for: Resourceful Contextual Bandits
Source: arXiv:1402.6779 source file (2015-07-31)
Supplement: Supplementary file 1 [file cbwk-supplement.tex]

\documentclass{article}

\usepackage{times}
\usepackage{mysetup,xspace}
\usepackage{mathrsfs}
\usepackage{verbatim}

\usepackage{algorithm}
\usepackage[noend]{algorithmic}

\usepackage{hyperref}
\usepackage{icml2014}
% macro for edits and comments, from David Kempe
\usepackage{color-edits}
\addauthor{ab}{green}   % ab for Ashwin
\addauthor{jl}{magenta} % jl for John
\addauthor{as}{red}     % as for Alex
% e.g. for Alex, provides \asedit{}, \ascomment{} and \asdelete{}.

%\newcommand{\fakeItem}[1][$\bullet$]{\vspace{2mm}\noindent{\bf #1}~~}

\author{Ashwinkumar Badanidiyuru
\footnote{Department of Computer Science, Cornell University, Ithaca NY, USA. Email: {\tt ashwinkumarbv@gmail.com}.
Parts of this work done during an internship at Microsoft Research New York.}
\and John Langford
\footnote{Microsoft Research, New York, NY, USA. Email: {\tt jcl@microsoft.com}.}
\and Aleksandrs Slivkins
\footnote{Microsoft Research, Mountain View, CA, USA. Email: {\tt slivkins@microsoft.com}.}
}

\begin{document}

\twocolumn[
\icmltitle{Resourceful Contextual Bandits \\ (supplementary material)}

% It is OKAY to include author information, even for blind
% submissions: the style file will automatically remove it for you
% unless you've provided the [accepted] option to the icml2014
% package.
\icmlauthor{Ashwinkumar Badanidiyuru}{ashwinkumarbv@gmail.com}
\icmladdress{Cornell University}
\icmlauthor{John Lnagford}{jcl@microsoft.com}
\icmladdress{Microsoft Research}
\icmlauthor{Alex Slivkins}{slivkins@microsoft.com}
\icmladdress{Microsoft Research}

% You may provide any keywords that you
% find helpful for describing your paper; these are used to populate
% the "keywords" metadata in the PDF but will not be shown in the document
\icmlkeywords{Bandits, Constraints}

\vskip 0.3in
]

\input{notation}

\begin{abstract}
We provide several discussions and proofs that are referred to from the full paper. 
\end{abstract}

\input{app-LP}

\input{app-applications}

\bibliographystyle{icml2014}
\bibliography{bib-abbrv-short,bib-slivkins,bib-bandits,bib-AGT,bib-random}
% A.S.: for short conference names: "bib-abbrv" -> "bib-abbrv-short".

\end{document}
